# Supplementary material for: Stacking, Strain, & Twist in 2D Materials Quantified by 3D Electron Diffraction
Source: arXiv:1905.11354 ancillary file (2019-05-28)
Supplement: Supplementary file 1 [file Supplemental_Materials.pdf]

# Supplemental Materials for: Stacking, Strain, & Twist in 2D Materials Quantified by 3D Electron Diffraction

Suk Hyun Sung,[1] Noah Schnitzer,[1] Lola Brown,[2] Jiwoong Park,[3,4,5] and Robert Hovden[1,6]
[1]*Department of Materials Science and Engineering, University of Michigan, Ann Arbor, Michigan 48109, USA*
[2]*Intel Electronics, Kiryat Gat 82109, Israel*
[3]*Department of Chemistry, University of Chicago, Chicago, Illinois 60637, USA*
[4]*Institute for Molecular Engineering, University of Chicago, Chicago, Illinois 60637, USA*
[5]*James Franck Institute, University of Chicago, Chicago, Illinois 60637, USA*
[6]*Applied Physics Program, University of Michigan, Ann Arbor, Michigan 48109, USA**
(Dated: May 27, 2019)

## I. EXPERIMENTAL METHODS

**Electron Diffraction:** Diffraction experiments on 2D materials were conducted in a TEM. Data on bilayer graphene (BLG) (Fig. 2) was acquired using an FEI Tecnai T12 operating at 80 keV. A portion of the BLG data first appeared in a report by Brown *et al.* [16]. Data on multilayer graphene (Fig. 6) were acquired on a JEOL 2010F operated at 200 keV. Data on $MoS_2$ (Fig. 5) were acquired using a JEOL 3100R05 operating at 80 keV.

**Data Processing:** Diffraction spots at every specimen tilt were characterized by first fitting a five parameter two-dimensional Gaussian and a constant background level to a windowed region about each peak. The integrated diffraction peak intensity was then determined and plotted to form a tilt-pattern.

## II. MATHEMATICAL FORMULATION OF 2D LATTICE

A 1D lattice with lattice constant $a$ can be represented as an infinite array of Dirac delta functions ($\sum_m \delta(x - ma)$), or more compactly as a 'Shah' function ($\text{Ш}_a(x)$). The Fourier transform of the 1D Shah function using the non-unitary, angular frequency convention (i.e $\mathcal{F}[\ ] = \int dx\ e^{-ikx}[\ ]$) is:

$$\mathcal{F}[\text{Ш}_a(x)] = \text{Ш}_b(k), \tag{1}$$

where $b$ is the reciprocal lattice constant. Note a normalization factor $\frac{2\pi}{a}$ has been included in reciprocal space Shah function, $\text{Ш}_b(k)$.

Expanding the definition, the 2D Shah function with two lattice vectors, $\mathbf{a_1}, \mathbf{a_2}$ ($\text{Ш}_{\mathbf{a}_1,\mathbf{a}_2}(\mathbf{r}_{xy})$) represents a 2D lattice:

$$\text{Ш}_{\mathbf{a_1},\mathbf{a_2}} = \sum_{m,n} \delta^2(\mathbf{r}_{xy} - (m\mathbf{a_1} + m\mathbf{a_2})). \tag{2}$$

The Fourier transform of the 2D Shah is $\text{Ш}_{\mathbf{b}_1,\mathbf{b}_2}(\mathbf{k_{xy}})$. Here $\mathbf{b_1}, \mathbf{b_2}$ are the reciprocal lattice vectors. This notation includes a normalization factor absorbed into the reciprocal Shah function, where the factor depends on the dimension of the function. The normalization factors are $\frac{2\pi}{a}, \frac{(2\pi)^2}{\Omega}, \frac{(2\pi)^3}{V}$ for the 1D, 2D and 3D cases, where $a, \Omega, V$ are the 1D, 2D, and 3D volumes of the real-space unit cell, respectively.

However, because the lattice is defined on a 2D plane, the real-space lattice points are infinite lines along $\hat{\mathbf{z}}$. To properly formulate a 2D planar lattice in 3D and place it in arbitrary z-position $z_0$, an additional delta function is necessary: ($\text{Ш}_{\mathbf{a}_1,\mathbf{a}_2}(\mathbf{r}_{xy})\delta(z - z_0)$). Applying the 3D Fourier transform, the reciprocal structure of the 2D lattice is:

$$\mathcal{F}[\text{Ш}_{\mathbf{a}_1,\mathbf{a}_2}(\mathbf{r}_{xy})\delta(z - z_0)] = e^{-ik_z z_0}\text{Ш}_{\mathbf{b}_1,\mathbf{b}_2}(\mathbf{k}_{xy}). \tag{3}$$

Therefore, the 3D reciprocal lattice of a 2D crystal is a 2D array of rods with phase associated with the $z$ position.

## III. PARAMETERIZING THE EWALD SPHERE IN TERMS OF SPECIMEN ORIENTATION

The Ewald sphere is most intuitively parameterized in terms of specimen orientation in spherical coordinates, where $\phi$ is the rotation angle of the specimen about the beam axis, and $\theta$ is the specimen tilt angle relative to the beam direction. The radius of the Ewald sphere is the wavenumber of the electron beam ($k_0$). A reciprocal space coordinate on the $k_z = 0$ plane $(k_x, k_y, 0)$ will be transformed as $k'_x = k_x - k_0 \sin(\theta)\cos(\phi)$, $k'_y = k_y - k_0 \sin(\theta)\sin(\phi)$, $k'_z = k_0 \cos(\theta)$. Thus, in Cartesian coordinates the Ewald sphere will cut through a reciprocal space rod at

$$k_z = k'_z - \sqrt{k_0^2 - {k'_x}^2 - {k'_y}^2} \tag{4}$$

and the in-plane radial distance to the reciprocal space origin is given by $k_\rho = \sqrt{k_x^2 + k_y^2}$

* hovden@umich.edu

## IV. EXTRACTING NUMBER OF LAYERS IN GRAPHENE FROM 2ND ORDER RODS

The three sublattices (A,B,C) of registered graphene have different phases associated with them ($\phi_A = 1 + e^{-\frac{2\pi i}{3}(h+k)}, \phi_B = e^{-\frac{2\pi i}{3}(h+k)} + e^{-\frac{4\pi i}{3}(h+k)}, \phi_C = 1 + e^{-\frac{4\pi i}{3}(h+k)}$), where $h$, $k$ are reciprocal lattice indices. For example, in the 2nd order rods (e.g. $h = 1$, $k = -1$), the phase terms simply equal constants ($\phi_{A,B,C} = 2$).

Placing a sublattice at a specific $z = z_0$ adds an extra phase of $e^{-ik_z z_0}$. Therefore adding N layers with equal interlayer spacing ($\lambda_L$) results in the typical finite size effect for a crystal, a complex magnitude of $2(1 + e^{-ik_z\lambda_L} + e^{-2ik_z\lambda_L} + ... + e^{-ik_z\lambda(N-1)})$, or more compactly $2\sum_{n=0}^{N-1}(e^{-ik_z\lambda_L})^n$. This geometric series can be expanded as $2\frac{1-e^{-ik_z\lambda_L N}}{1-e^{-ik_z\lambda_L}}$. The measured intensity is equal to the magnitude squared:

$$I = 4\frac{\sin^2 \frac{1}{2}k_z\lambda_L N}{\sin^2 \frac{1}{2}k_z\lambda_L} \tag{5}$$

The numerator reaches zero at $k_z = \frac{2\pi m}{\lambda_L N}, m \in \mathbb{Z}$. If we choose $m = 1$ (the first minimum), the intensity is also zero with the exception of $N = 1$ (trivial SLG case). Therefore, the first minimum of the 2nd order Bragg rods of multilayer graphene occurs at $k_z = \frac{2\pi}{\lambda_L N}$

When tilted along the first order peaks by an angle $\theta$, the diffraction plane slices the 2nd order rods at $k_z = b_g\sqrt{3}\tan\theta$, where $b_g = \frac{4\pi}{a_g\sqrt{3}}$ and $a_g$ is the lattice constant of graphene. Substituting, we can arrive at $N = \frac{a_g}{2\lambda_L \tan\theta}$. Using $a_g = 2.46$ Å, $\lambda_L = 3.346$Å, $\tan\theta \approx \theta$ (in radians), we arrive at:

$$N \approx \frac{21}{\theta(deg)} \tag{6}$$

## V. MEASURING THICKNESS IN MULTILAYER GRAPHENE FROM 2ND ORDER BRAGG RODS

The maxima of measured intensity (Eq. 5) is at $k_z = \frac{(2m+1)\pi}{\lambda_L N}$:

$$I_m = \frac{4}{\sin^2 \frac{(2m+1)\pi}{2N}} \tag{7}$$

The relative intensity these maxima depends only on the number of layers, N.

$$\frac{I_m}{I_{m'}} = \frac{\sin^2 \frac{(2m'+1)\pi}{2N}}{\sin^2 \frac{(2m+1)\pi}{2N}} \tag{8}$$

Looking at this ratio for $(m, m') = (1, 2)$, we compare the maximum between the 1st and 2nd minima, and the maximum between the 2nd and 3rd minima:

$$\frac{I_1}{I_2} = \frac{\sin^2 \frac{5\pi}{2N}}{\sin^2 \frac{3\pi}{2N}} \tag{9}$$

Comparison of this expression with experimental data determines the number of layers in samples.

## VI. EXTRACTING FRACTION OF SUBLATTICES OF GRAPHENE

From Supplemental Section IV, the phase associated with each of the sub-lattices of registered graphene are $\phi_A = 1+e^{-\frac{2\pi i}{3}(h+k)}, \phi_B = e^{-\frac{2\pi i}{3}(h+k)} + e^{-\frac{4\pi i}{3}(h+k)}, \phi_C = 1 + e^{-\frac{4\pi i}{3}(h+k)}$. Looking at $k_z = 0$, there is no phase term related to the out-of-plane; real-space equivalence of projected view.

Therefore the total added phase at $k_z$ with $N$ total layers and $N_A, N_B, N_C$ layers for each sublattice, is:

$$N_A(1 + e^{-\frac{2\pi i}{3}(h+k)}) + N_B(e^{-\frac{2\pi i}{3}(h+k)} + e^{-\frac{4\pi i}{3}(h+k)}) + N_C(1 + e^{-\frac{4\pi i}{3}(h+k)}) \tag{10}$$

For the 2nd order rods ($h + k = 0$), the phase term reduces to $2(N_A + N_B + N_C) = 2N$, resulting in a magnitude squared intensity of $4N^2$ for the 2nd order peaks at $k_z = 0$.

For the 1st order peaks ($h+k = 1$), the squared intensity reduces to phase term reduces to $N^2 - 3(N_A N_B + N_A N_C + N_B N_C)$. Defining fractional sublattice number $n_i \equiv N_i/N$, the relative intensity of 1st order to 2nd order is: $\frac{1-3(N_A N_B+N_A N_C+N_B N_C)}{N^2} = \frac{1-3(n_A n_B+n_A n_C+n_B n_C)}{4}$

The scattering factor of the carbon atom is about 4.5 times greater at $\Gamma_1$ site than at $\Gamma_2$. Taking this into account, the relative intensity is then:

$$I_{1st/2nd} \approx 1 - 3(n_A n_B + n_A n_C + n_B n_C). \tag{11}$$

Therefore, the rhombohedral stacking (ABCAB-CABC..., i.e $n_A = n_B = n_C = \frac{1}{3}$) has $I_{1st/2nd} = 0$, while the Bernal stacking (ABABAB..., i.e $n_A = n_B\frac{1}{2}, n_C = 0$) has $I_{1st/2nd} \approx 0.25$

## VII. EVOLUTION OF BRAGG RODS WITH THICKNESS

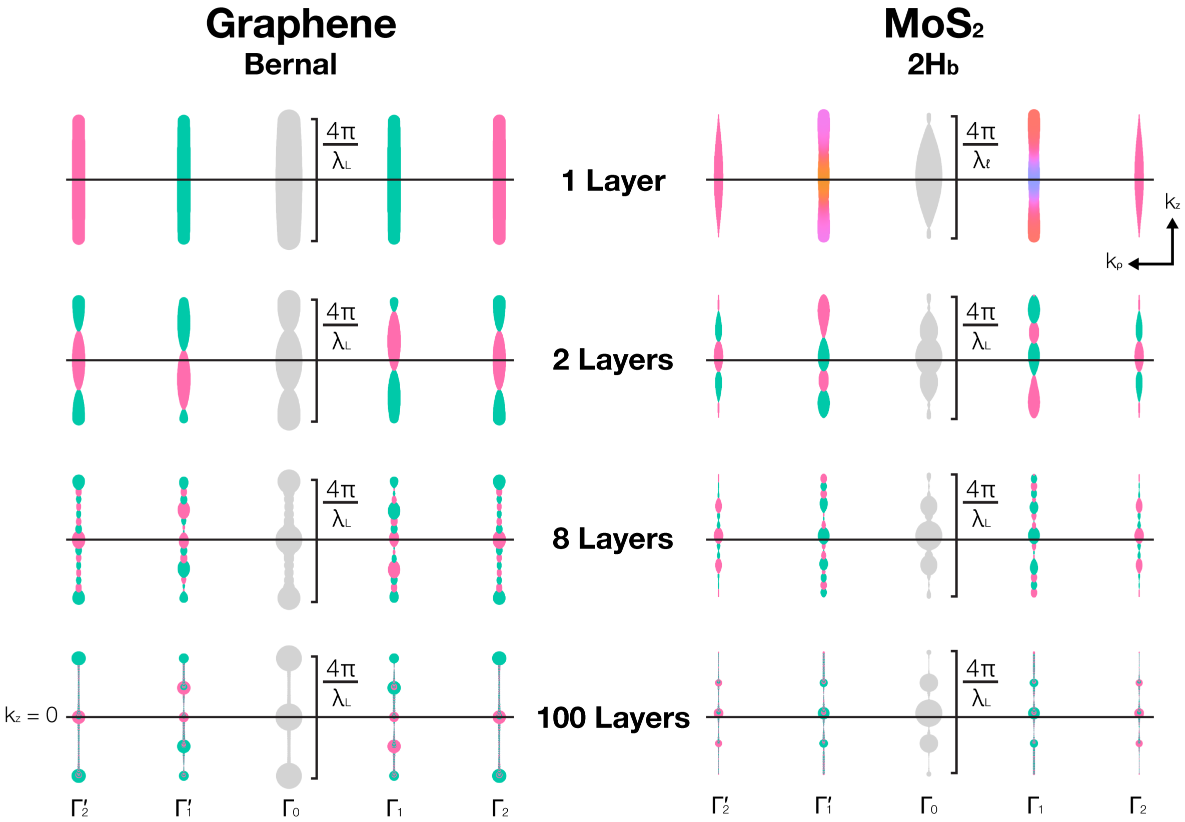


FIG. S1. **Evolution of Bragg Rods with Thickness.** Sideview of the Bragg rods ($\Gamma_0$, $\Gamma_1$, $\Gamma_2$) quantitatively illustrates the structure in $k$-space. With additional layers the rods converge into Bragg peaks. The thickness and color indicates complex magnitude and phase respectively.

## VIII. ATLAS OF 3D RECIPROCAL STRUCTURE OF 2D MATERIALS

### A. Multilayer Graphene

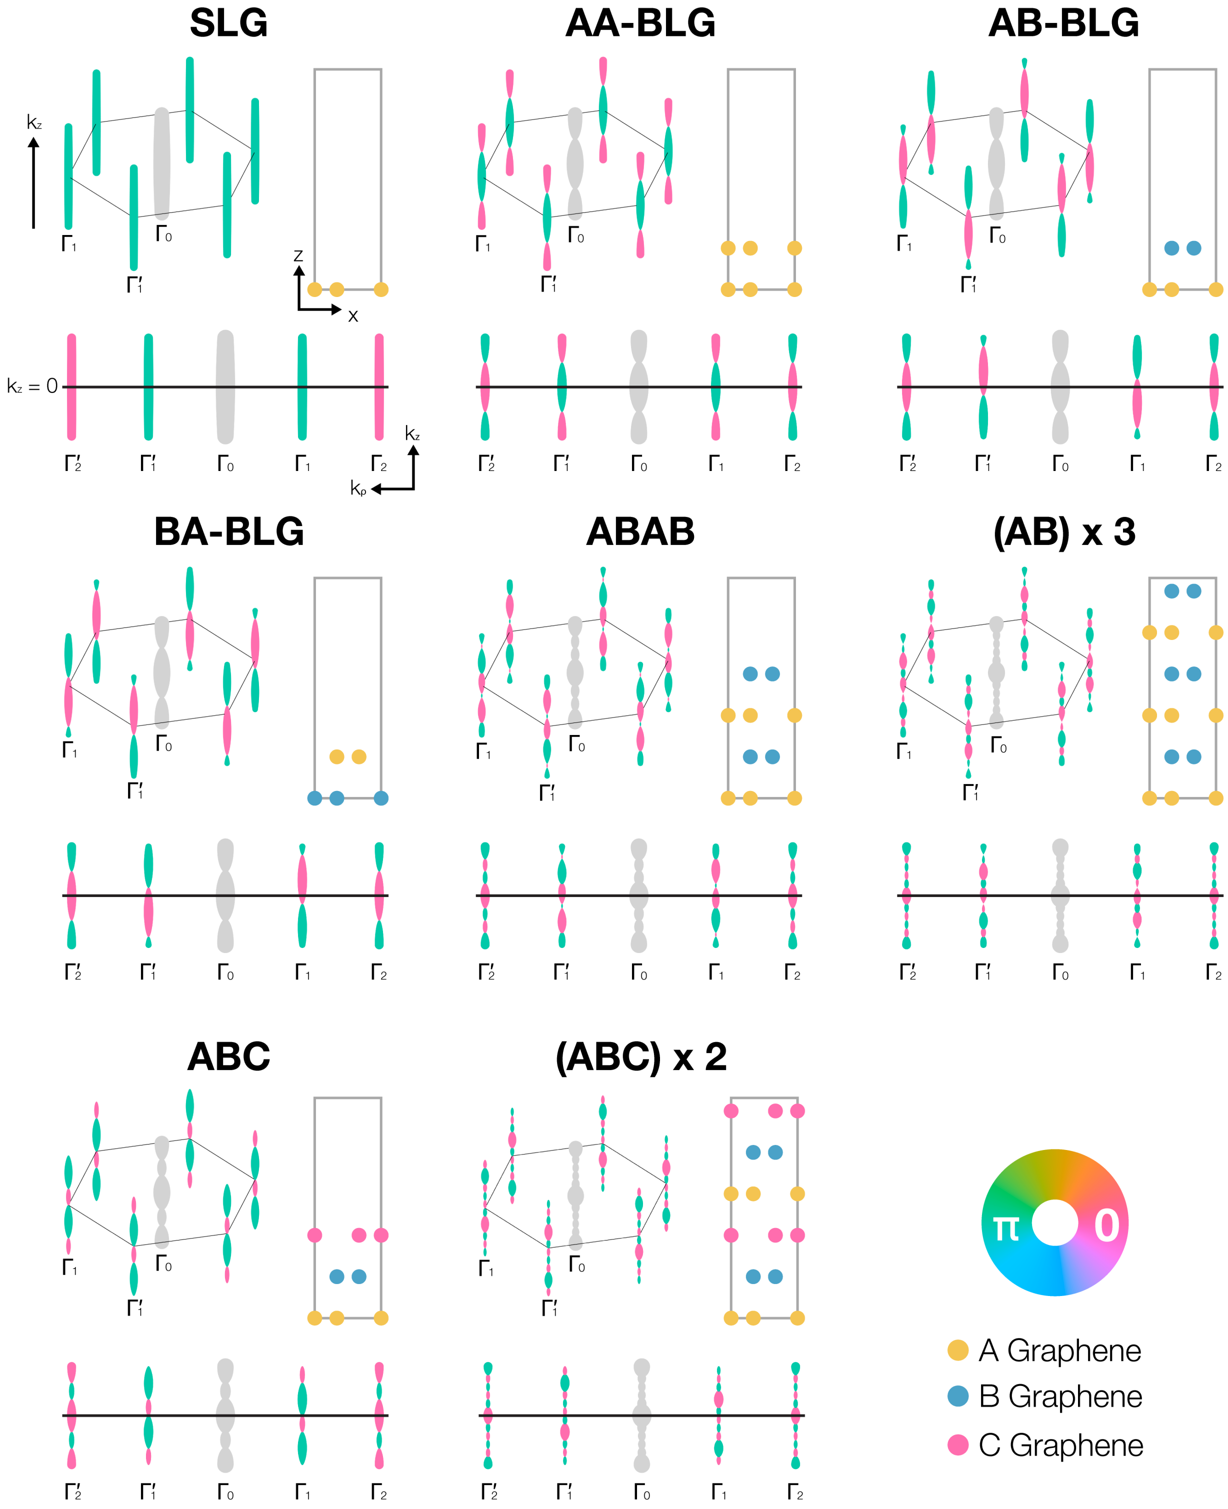


FIG. S2. **3D Reciprocal Structure of Multilayer Graphene.** The Bragg rods ($\Gamma_0$, $\Gamma_1$) are shown in 3D alongside a real-space <100> projection of the crystal stacking order. Below, a sideview of the Bragg rods ($\Gamma_0$, $\Gamma_1$, $\Gamma_2$) quantitatively illustrates the structure in $k$-space. Bragg rods have thickness and color indicating the complex magnitude and phase respectively.

## B. Transition Metal Dichalcogenides

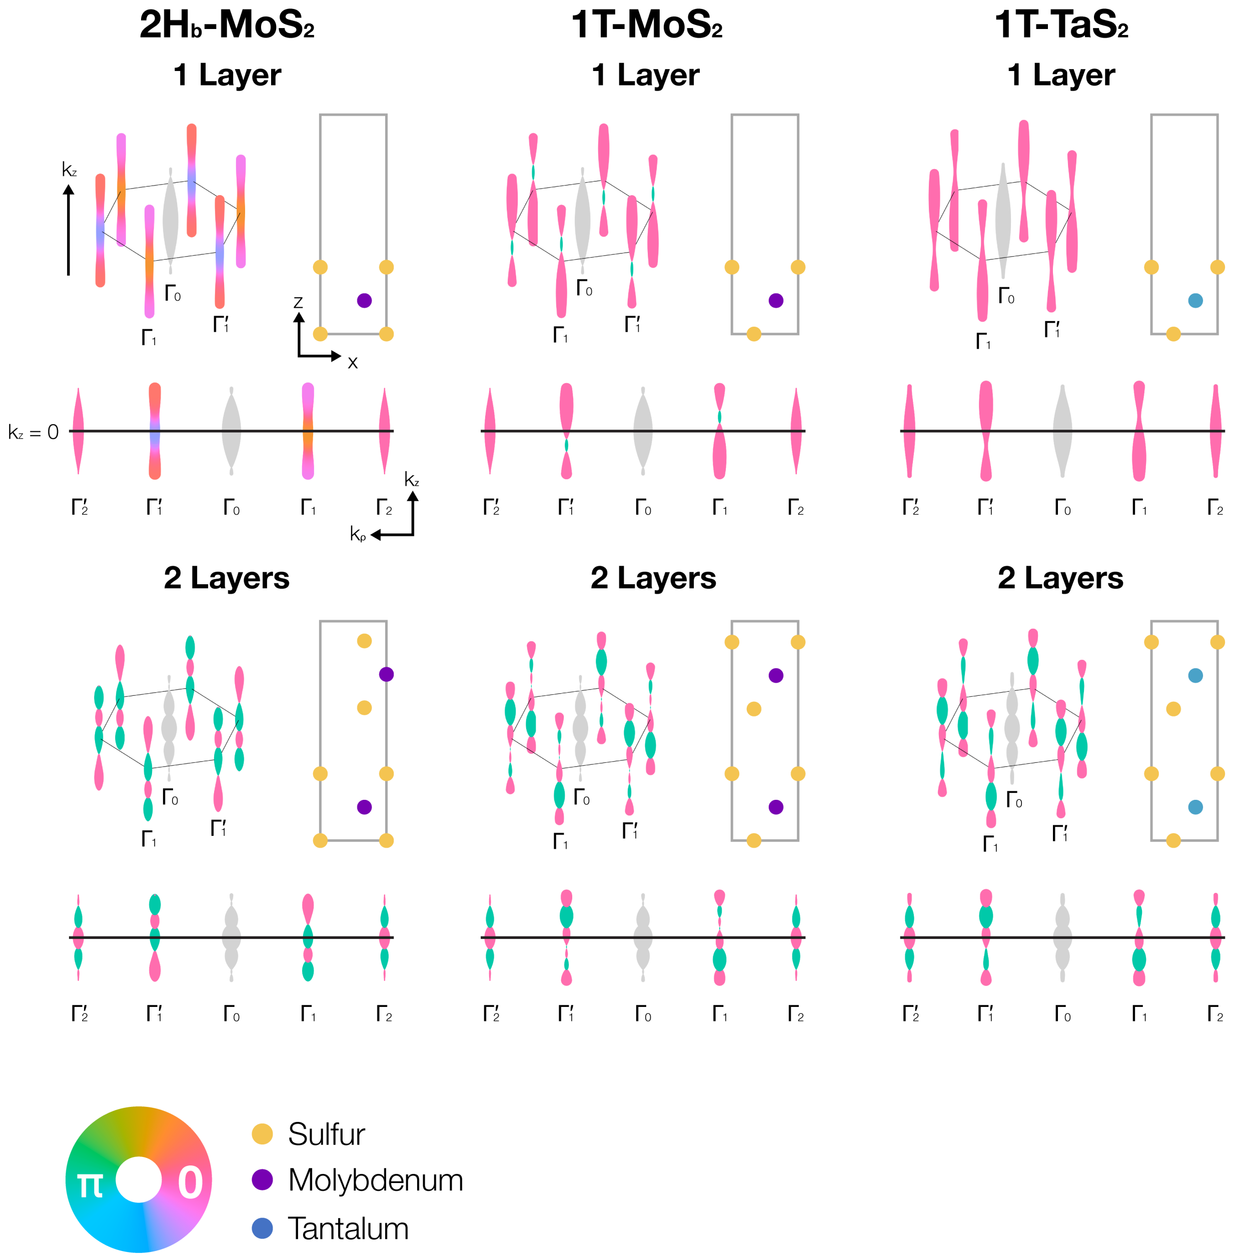


FIG. S3. **3D Reciprocal Structure of mono- and bi-layer TMDs.** The Bragg rods ($\Gamma_0$, $\Gamma_1$) are shown in 3D alongside a real-space <100> projection of the crystal stacking order. Below, a sideview of the Bragg rods ($\Gamma_0$, $\Gamma_1$, $\Gamma_2$) quantitatively illustrates the structure in $k$-space. Bragg rods have thickness and color indicating the complex magnitude and phase respectively.

## IX. ATLAS OF TILT-PATTERNS

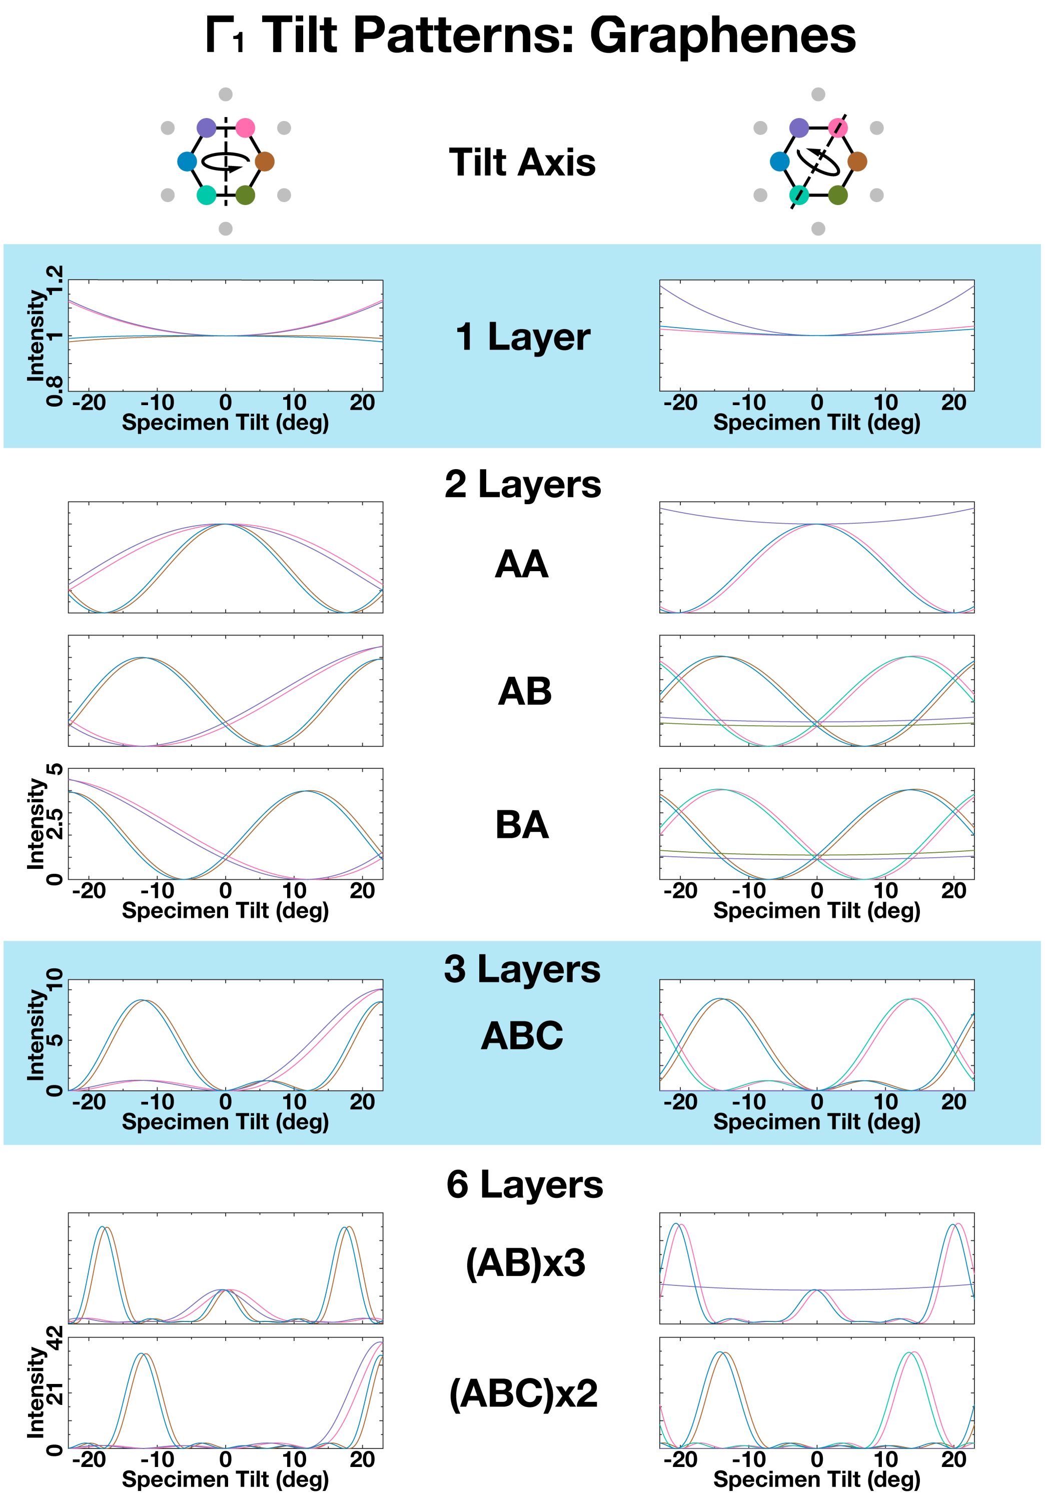


FIG. S4. **Simulated diffraction tilt-pattern of multilayer graphene.** The axis of rotation illustrated *top* shows the principle axis that passes through second order $\Gamma_2$ (*left column*) and first order $\Gamma_1$ (*right column*) Bragg peaks. The tilt patterns are generated for first order peaks only. The small splitting of Friedel pairs in each curve corresponds to a 200 keV electron beam voltage.

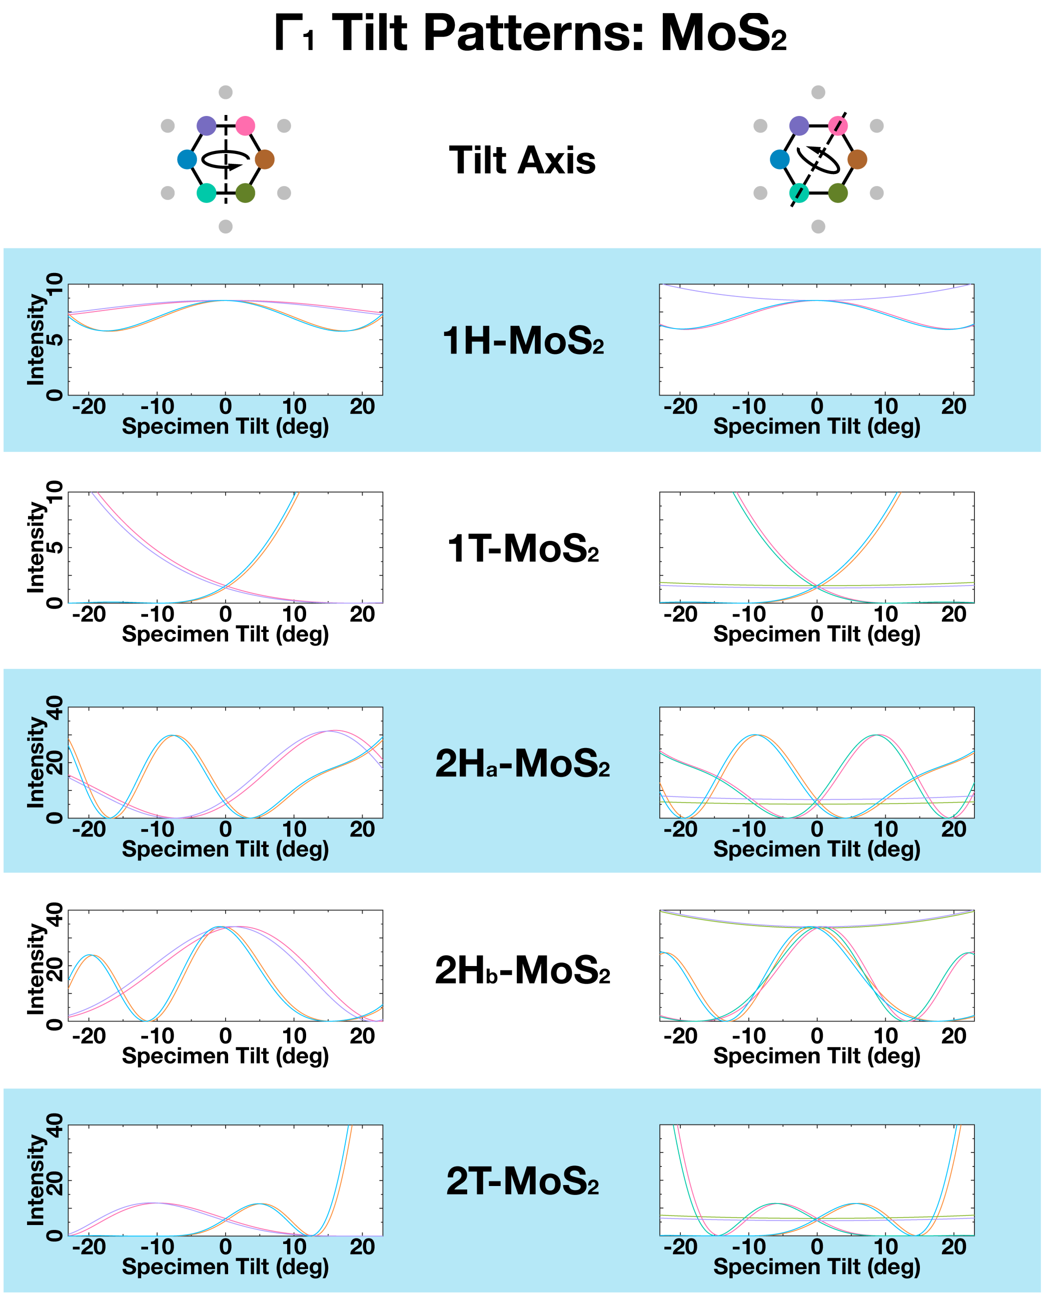


FIG. S5. **Simulated diffraction tilt-patterns of single and bilayer $MoS_2$ and polytypes thereof.** The axis of rotation illustrated *top* shows the principle axis that passes through second order $\Gamma_2$ (*left column*) and first order $\Gamma_1$ (*right column*) Bragg peaks. The tilt patterns are generated for first order peaks only. The small splitting of Friedel pairs in each curve corresponds to a 200 keV electron beam voltage.

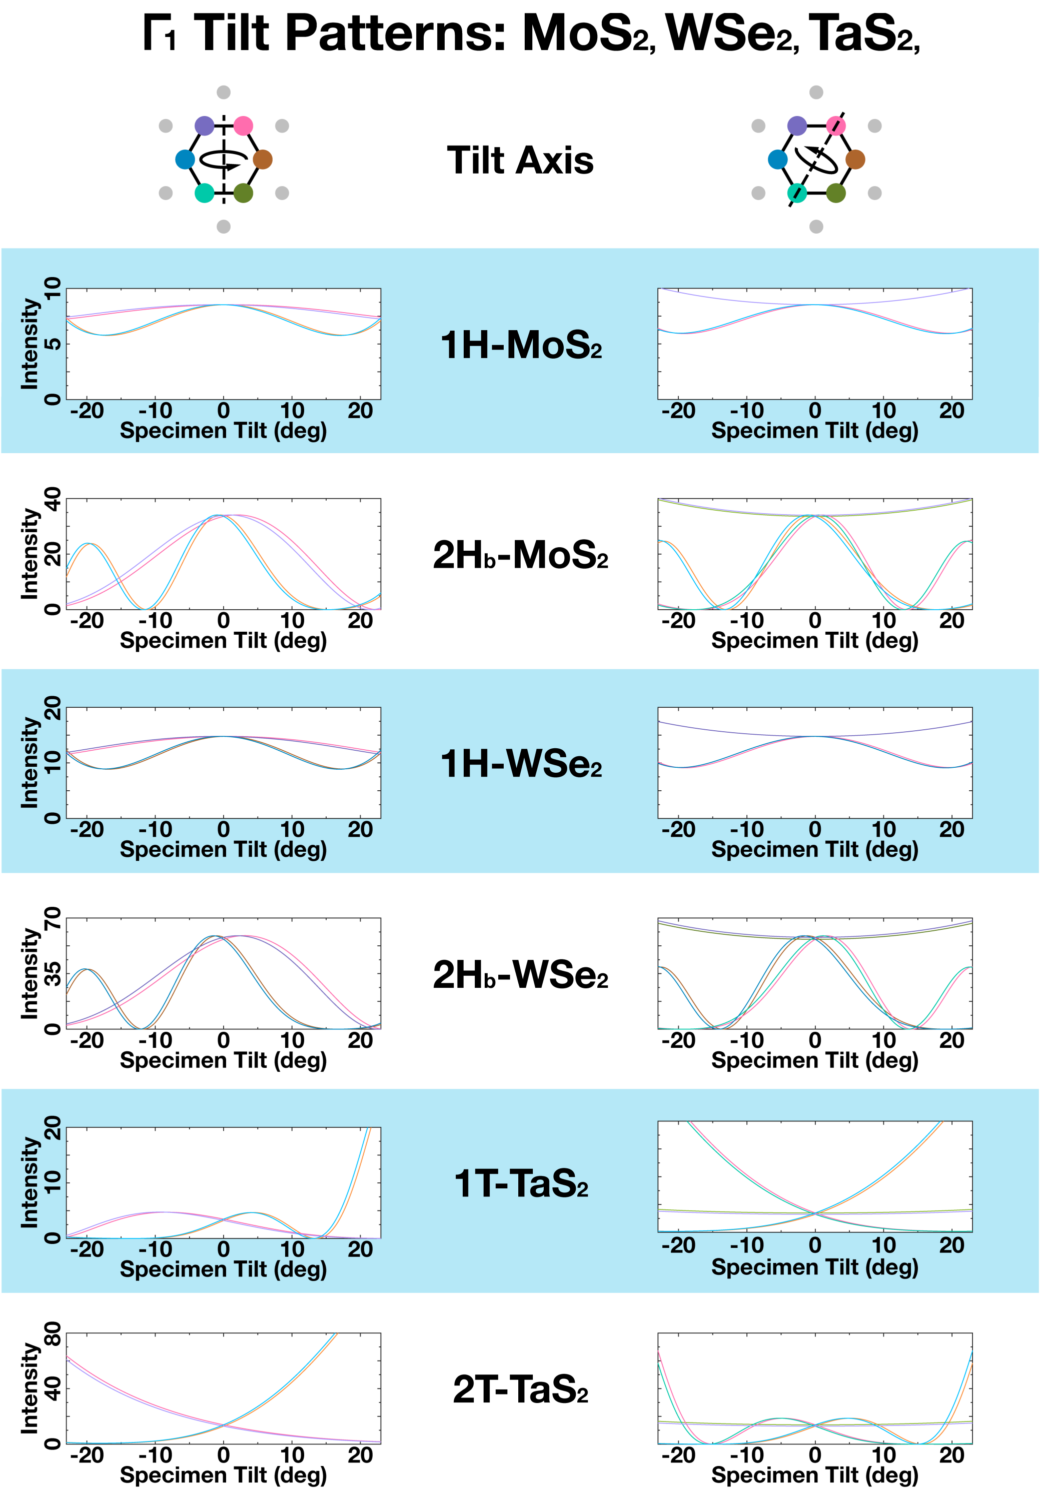


FIG. S6. **Simulated diffraction tilt-patterns of various $MoS_2$, $WSe_2$, $TaS_2$ and polytypes thereof.** The axis of rotation illustrated *top* shows the principle axis that passes through second order $\Gamma_2$ (*left column*) and first order $\Gamma_1$ (*right column*) Bragg peaks. The tilt patterns are generated for first order peaks only. The small splitting of Friedel pairs in each curve corresponds to a 200 keV electron beam voltage.

## X. KINEMATIC AND EXPERIMENTAL BRAGG RODS INTENSITIES OVER $\mathbf{K_z}$

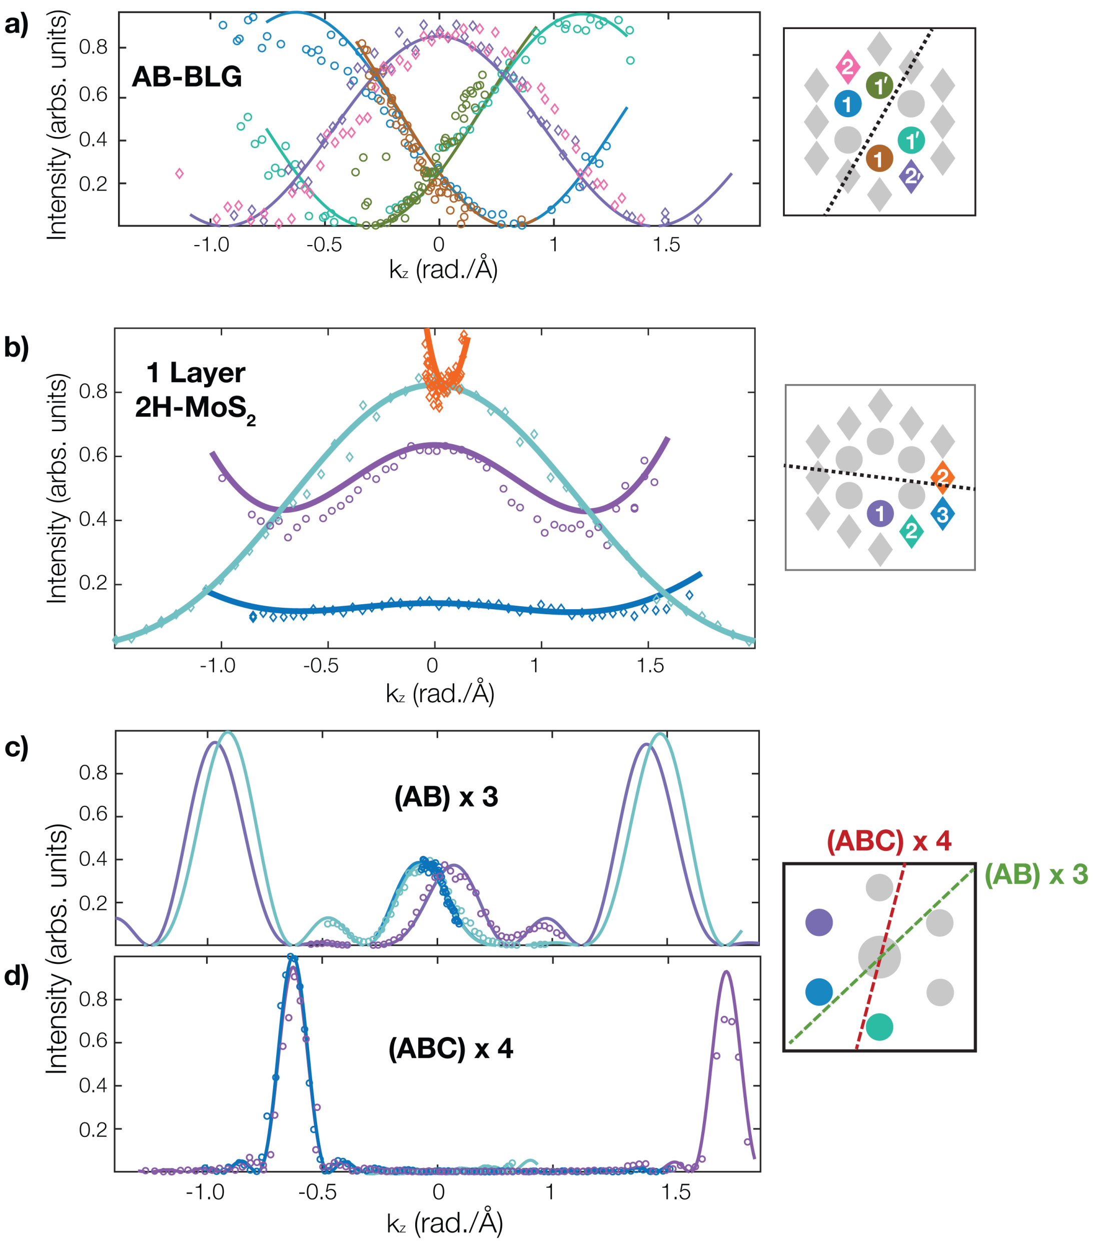


FIG. S7. **Bragg rod intensities over $\mathbf{k_z}$.** Kinematic (—) and experimental (○, ◊) diffraction tilt-patterns of a) BLG, b) monolayer 2H-$MoS_2$, c) (AB)x3 stacked graphene, d) (ABC)x4 stacked graphene plotted against $k_z$. Plotting over $k_z$ quantitatively illustrates the periodicities of the structure; however, the extent measured in $k_z$ varies from rod to rod depending on the distance from the tilt axis.
